# Supplementary material for: Size control of Charge-Orbital Order in Half-Doped Manganite, La$_{0.5}$Ca$_{0.5}$MnO$_3$
Source: arXiv:1110.2912 source file (2011-10-13)
Supplement: Supplementary file 1 [file supplementary.pdf]

# Size control of Charge-Orbital Order in Half-Doped Manganite, $La_{0.5}Ca_{0.5}MnO_3$

Hena Das[1], G. Sangiovanni[2], A. Valli[2], K. Held[2] and T. Saha-Dasgupta[1]
[1] *S.N. Bose National Centre for Basic Sciences, Kolkata 700098, India and*
[2] *Institute for Solid State Physics, Vienna University of Technology, 1040 Wien, Austria*

PACS numbers: 68.65.-k,71.27.+a,71.15.Mb

## I. DETAILS OF STRUCTURAL PARAMETERS OF VARIOUS STRUCTURES

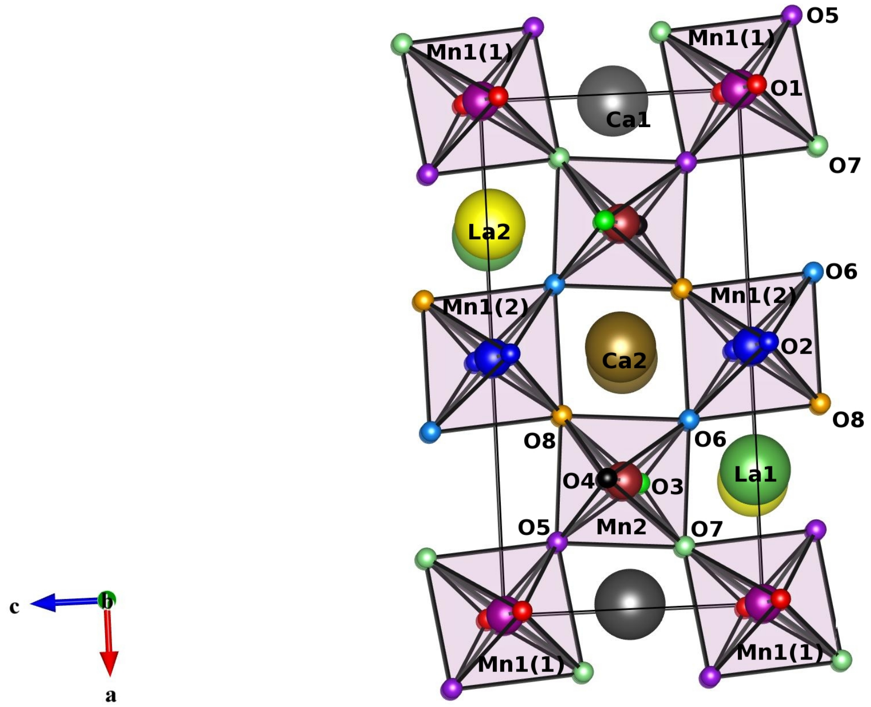


FIG. 1: The monoclinic unit cell. The different inequivalent La, Ca, Mn and O atoms are colored differently, as well as marked.

TABLE I: The lattice constants and atomic positions of various structures used for calculations. The lattice parameters are given for monoclinic unit cell, based on a doubled cell (2 $a \times b \times c$) compared to that given in the main text.

| | $S_{ex}$ | | | $S_{bulk}$ | | | $S_{model}$ | | | $S_{press}$ | | |
|---|---|---|---|---|---|---|---|---|---|---|---|---|
| a | 10.90 | | | 10.95 | | | 10.57 | | | 10.69 | | |
| b | 7.52 | | | 7.58 | | | 7.48 | | | 7.40 | | |
| c | 5.47 | | | 5.48 | | | 5.39 | | | 5.35 | | |
| $\beta$ | 90.0 | | | 89.79 | | | 90.0 | | | 89.79 | | |
| | x | y | z | x | y | z | x | y | z | x | y | z |
| Mn1(1) | 0.0 | 0.0 | 0.0 | 0.0 | 0.0 | 0.0 | 0.0 | 0.0 | 0.0 | 0.0 | 0.0 | 0.0 |
| Mn1(2) | 0.5 | 0.0 | 0.0 | 0.5 | 0.0 | 0.0 | 0.5 | 0.0 | 0.0 | 0.5 | 0.0 | 0.0 |
| Mn2 | 0.25 | 0.0 | 0.482 | 0.252 | 0.0 | 0.526 | 0.755 | 0.006 | 0.481 | 0.249 | -0.001 | 0.513 |
| La1 | 0.26 | 0.25 | -0.006 | 0.263 | 0.25 | 0.013 | 0.258 | 0.25 | -0.008 | 0.26 | 0.25 | 0.012 |
| La2 | 0.76 | 0.25 | 0.014 | 0.761 | 0.25 | -0.018 | 0.764 | 0.25 | 0.017 | 0.759 | 0.25 | -0.016 |
| Ca1 | 0.010 | 0.25 | 0.496 | 0.017 | 0.25 | 0.507 | 0.019 | 0.25 | 0.476 | 0.014 | 0.25 | 0.507 |
| Ca2 | 0.51 | 0.25 | 0.496 | 0.512 | 0.25 | 0.509 | 0.501 | 0.25 | 0.498 | 0.511 | 0.25 | 0.507 |
| O1 | -0.005 | 0.25 | -0.065 | 0.010 | 0.25 | -0.072 | 0.0 | 0.25 | -0.069 | -0.004 | 0.25 | 0.072 |
| O2 | 0.495 | 0.25 | -0.065 | 0.501 | 0.25 | -0.077 | 0.491 | 0.25 | -0.069 | 0.509 | 0.25 | 0.072 |
| O3 | 0.245 | 0.25 | 0.547 | 0.269 | 0.25 | 0.595 | 0.264 | 0.25 | 0.567 | 0.240 | 0.25 | 0.452 |
| O4 | 0.745 | 0.25 | 0.583 | 0.759 | 0.25 | 0.549 | 0.764 | 0.25 | 0.567 | 0.739 | 0.25 | 0.430 |
| O5 | 0.138 | 0.034 | 0.217 | 0.144 | -0.033 | -0.196 | -0.142 | 0.041 | 0.215 | -0.138 | -0.032 | 0.211 |
| O6 | 0.638 | 0.034 | 0.253 | 0.360 | 0.031 | 0.257 | 0.636 | -0.023 | -0.249 | 0.363 | -0.025 | 0.239 |
| O7 | 0.118 | -0.034 | 0.707 | 0.118 | 0.041 | 0.314 | -0.113 | -0.049 | 0.717 | 0.113 | -0.036 | 0.286 |
| O8 | 0.618 | -0.034 | 0.743 | 0.390 | -0.047 | 0.737 | 0.606 | 0.039 | -0.716 | 0.387 | 0.044 | 0.738 |

TABLE II: Various Mn-O bondlengths and Mn-O-Mn bondangles in different structures.

| | $S_{ex}$ | $S_{bulk}$ | $S_{model}$ | $S_{press}$ |
|---|---|---|---|---|
| Bond lengths (Å) | | | | |
| Mn1(1)-O7 | 2.067 | 2.180 | 1.971 | 1.978 |
| Mn1(1)-O5 | 1.925 | 1.925 | 1.922 | 1.869 |
| Mn1(1)-O1 | 1.913 | 1.940 | 1.907 | 1.890 |
| Mn1(2)-O6 | 2.055 | 2.089 | 1.974 | 1.949 |
| Mn1(2)-O8 | 1.918 | 1.915 | 1.919 | 1.881 |
| Mn1(2)-O2 | 1.913 | 1.942 | 1.909 | 1.892 |
| Mn2-O7 | 1.914 | 1.900 | 1.932 | 1.907 |
| Mn2-O8 | 1.914 | 1.941 | 1.915 | 1.937 |
| Mn2-O5 | 1.915 | 1.939 | 1.818 | 1.911 |
| Mn2-O6 | 1.915 | 1.904 | 1.936 | 1.907 |
| Mn2-O3 | 1.913 | 1.942 | 1.943 | 1.889 |
| Mn2-O4 | 1.913 | 1.943 | 1.886 | 1.872 |
| Bond angles (degree) | | | | |
| $\widehat{Mn1(1)-O7-Mn2}$ | 161.64 | 157.15 | 155.10 | 160.76 |
| $\widehat{Mn1(1)-O5-Mn2}$ | 160.96 | 156.68 | 156.98 | 159.88 |
| $\widehat{Mn1(2)-O6-Mn2}$ | 163.61 | 164.14 | 167.03 | 165.89 |
| $\widehat{Mn1(2)-O8-Mn2}$ | 163.06 | 155.25 | 154.49 | 157.76 |
| $\widehat{Mn1(1)-O1-Mn1(1)}$ | 158.32 | 155.46 | 157.60 | 156.35 |
| $\widehat{Mn1(2)-O2-Mn1(2)}$ | 158.32 | 154.73 | 156.90 | 155.75 |
| $\widehat{Mn2-O4-Mn2}$ | 158.32 | 154.56 | 150.94 | 159.55 |
| $\widehat{Mn2-O3-Mn2}$ | 158.32 | 154.68 | 160.59 | 159.18 |

## II. CONSTRUCTION OF $S_{model}$

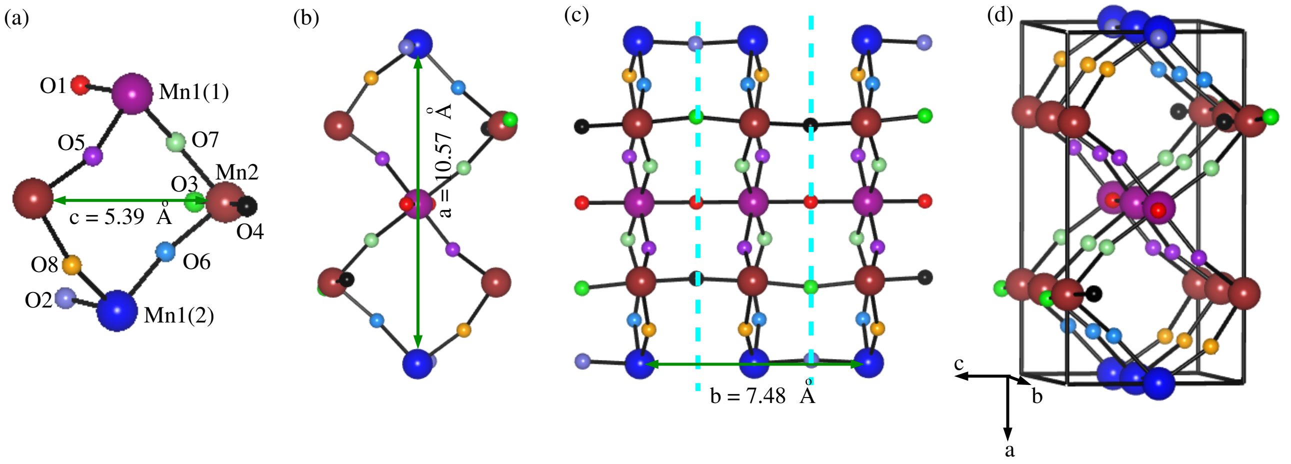


FIG. 2: (a) Step I: Sructural unit chosen from $S_{nano}$. The chosen unit already defines the lattice parameter, $c$. (b) Step II: Apply inversion about Mn1(1) atom, to define the lattice parameter $a$. (c) Step III: Apply mirror reflections passing through apical oxygens (marked as dashed lines) to define the lattice parameter $b$. (d) The fully constructed unit cell of $S_{model}$. La/Ca atoms are not shown for clarity.
